# Supplementary material for: Anomalous thermoelectric transport phenomena from interband electron-phonon scattering
Source: arXiv:2103.06558 ancillary file (2021-03-11)
Supplement: Supplementary file 1 [file HH_supplementary.pdf]

# Anomalous thermoelectric transport phenomena from interband electron-phonon scattering
# - Supplementary Material -

Natalya S. Fedorova,[1,2,*] Andrea Cepellotti,[1] and Boris Kozinsky[1,3,†]

[1] *Materials Intelligence Research group, John A. Paulson School of Engineering and Applied Sciences, Harvard University, 29 Oxford Street, Cambridge, MA 02138, USA*
[2] *Ferroic Materials for Transducers group, Materials Research and Technology Department, Luxembourg Institute of Science and Technology, 5 Avenue des Hauts-Fourneaux, L-4362 Esch/Alzette, Luxembourg*
[3] *Robert Bosch LLC Research and Technology Center, Cambridge, MA 02139, USA*

## I. CRYSTAL STRUCTURE OF HALF-HEUSLER MATERIALS

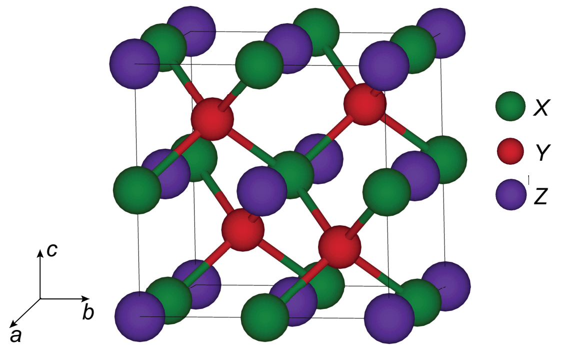


Figure 1. Crystal structure of half-Heusler (HH) systems. HH compound formula is $XYZ$, where $X$ is a transition metal, noble metal or rare-earth ion, $Y$ is a transition or noble metal and $Z$ is a main group element.

## II. COMPUTATIONAL DETAILS

All calculations of structural, electronic and vibrational properties of considered HHs have been performed using DFT[1,2], and DFPT[3] as implemented in Quantum ESPRESSO package[4,5]. We employ the generalized gradient approximation for the exchange-correlation functional in the form introduced by Perdew, Burke and Ernzerhof[6], optimized norm-conserving Vanderbilt pseudopotentials[7] and a plane wave basis set with wavefunction cutoff energy of 90 Ry. Spin-orbit coupling is not included in our calculations.

The crystal structures of TaFeSb and ZrNiSn have been optimized using a Γ-centered $8 \times 8 \times 8$ Monkhorst-Pack **k**-point grid and reducing the stress tensor components to values smaller than 0.1 kbar. We find optimized lattice parameters of $a = 5.958$ Å and 6.153 Å for TaFeSb and ZrNiSn respectively, which well compare with the experimental values of $a = 5.938$ Å[8] and $a = 6.115$ Å[9].

For computing transport coefficients, we use the rigid band approximation, i.e. the hypothesis that small doping concentrations only change the chemical potential but not the crystal band structure.

In order to obtain transport coefficients within the CRT approximation, we first compute the *ab initio* charge density using a Γ-centered $8 \times 8 \times 8$ **k**-point grid and the electronic band structure using Γ-centered $40 \times 40 \times 40$ **k**-point grid. Next, we interpolate the band structure on 5 times finer **k**-grid using Fourier interpolation and integrate transport coefficients with the software Boltztrap[10]. Unless specified otherwise, we (arbitrarily) set the relaxation time to $\tau = 10$ fs. Taking advantage of the cubic symmetry of the crystals, all plots refer to just the trace-average of transport coefficients tensors.

To compute the electron relaxation times within the EPA approximation[11] and the corresponding transport coefficients, we first obtain the charge density, phonon frequencies and electron-phonon matrix elements using Γ-centered $8 \times 8 \times 8$ **k**- and **q**-point grids. Next, we average the electron-phonon matrix elements using the moving least squares (MLS) averaging procedure[12] with energy bins of size 0.3 eV (10 bins in the valence and 10 bins in the conduction bands). The smoothing scale $\sigma_{Gauss}$ of the Gaussian function in EPA-MLS method is set to 0.5 eV. Then, we calculate

the band structure using a Γ-centered $40 \times 40 \times 40$ k-point mesh. Finally, we use a custom version of the software BoltzTraP to interpolate the band structure on 5 times finer k-grid using Fourier interpolation, as well as to calculate the energy-dependent lifetimes and the electronic transport coefficients.

To obtain the electron lifetimes and transport properties using the Wannier interpolation method[13], we calculate the electronic band structure, phonon frequencies and electron-phonon matrix elements using Γ-centered $8 \times 8 \times 8$ **k**- and **q**-point grids. Then, we interpolate these quantities on $56 \times 56 \times 56$ **k**- and **q**-point grids for TaFeSb and $48 \times 48 \times 48$ for ZrNiSn using the EPW software[14,15]. Finally, we calculate the electron lifetimes as well as electronic transport coefficients using a privately developed code.

## III. ELECTRONIC TRANSPORT PROPERTIES OF TaFeSb AND ZrNiSn

### A. TaFeSb

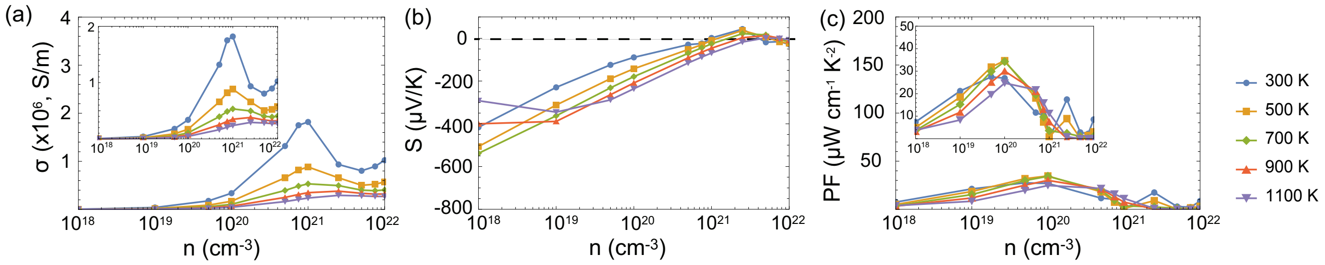


Figure 2. Electronic transport properties of n-type TaFeSb calculated using the Wannier interpolation method and shown as functions of carrier concentration $n$. We show the electrical conductivity $\sigma$ in panel (a), the Seebeck coefficient $S$ in (b) and the power factor PF in (c). Insets are magnifications of the same plots. Curve colors correspond to different temperatures in the range 300 - 1100 K.

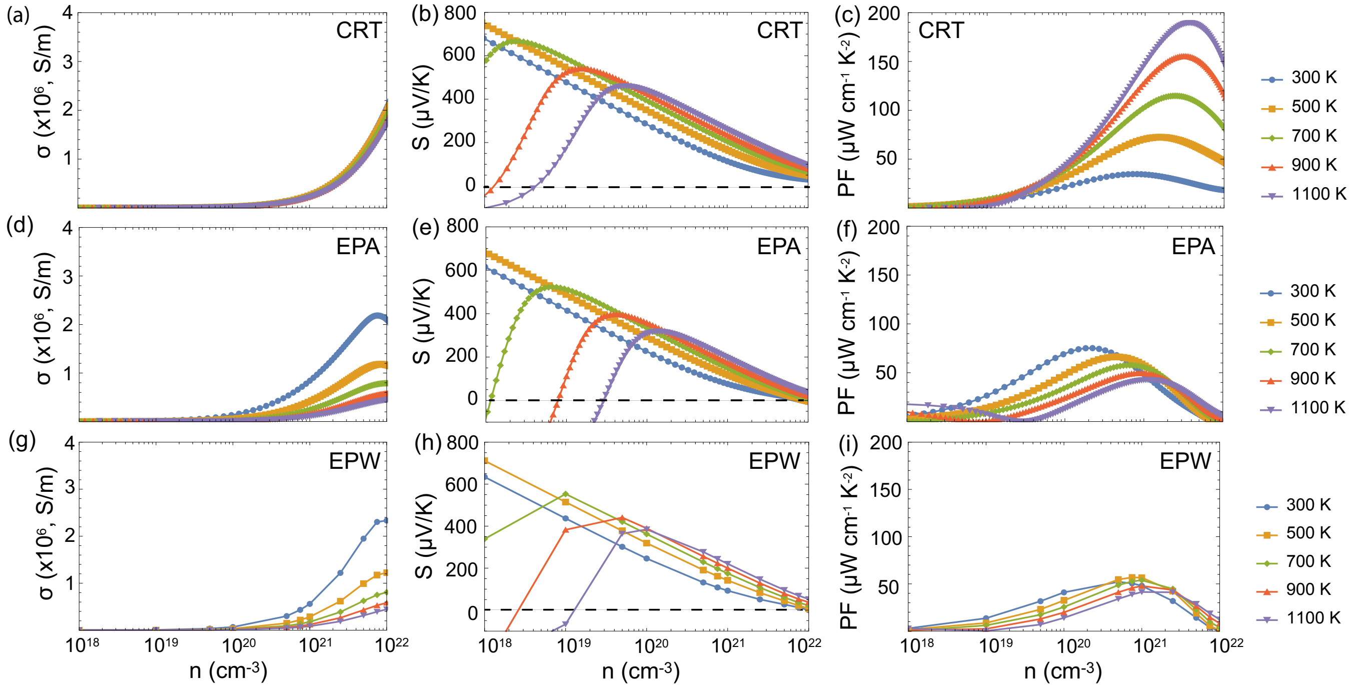


Figure 3. Electronic transport properties of p-type TaFeSb as functions of carrier concentration $n$. Panels (a), (b) and (c): transport coefficients (electrical conductivity $\sigma$, Seebeck coefficient $S$ and power factor $\sigma S^2$) calculated using the CRT approximation. Panels (d), (e), and (f): estimates of transport coefficients using the EPA approximation. Panels (g), (h), and (i): transport coefficients obtained using the Wannier-interpolation method. Different colors of curves correspond to different temperatures in the range 300 - 1100 K. As commented in Sec. III.A.4 of the main text, the Seebeck coefficient is predicted similarly by all methods. However, for electrical conductivity and thus the power factor, the CRT approximation neglects the noticeable impact of the temperature dependence of lifetimes.

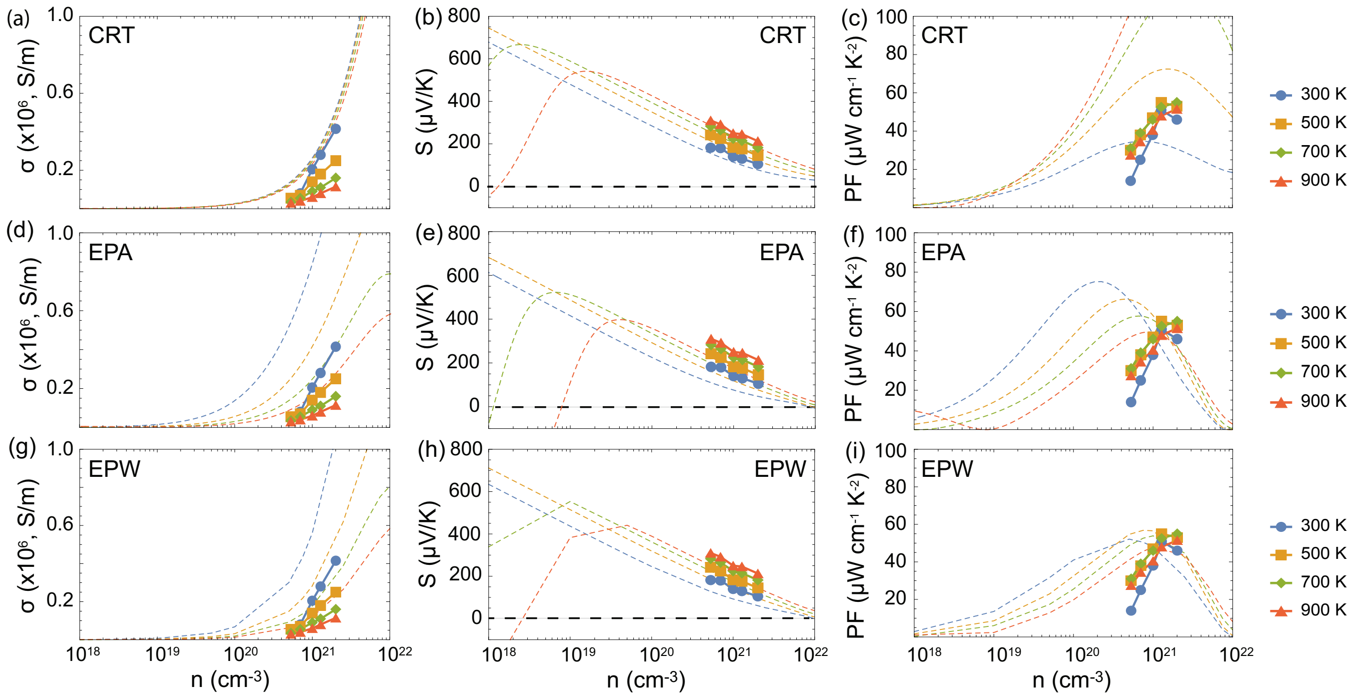


Figure 4. Comparison of the experimentally measured and this work's calculated electronic transport properties of p-type TaFeSb. Experimental data is shown as solid lines, and calculated data as dashed lines. The top row shows the electrical conductivity $\sigma$, the Seebeck coefficient $S$ and the power factor PF, respectively, calculated using the CRT approximation. Middle row: transport properties computed with the EPA approximation. Bottom row: transport properties computed using the Wannier-interpolation method. Curve colors tag different temperatures in the range 300 - 1100 K.

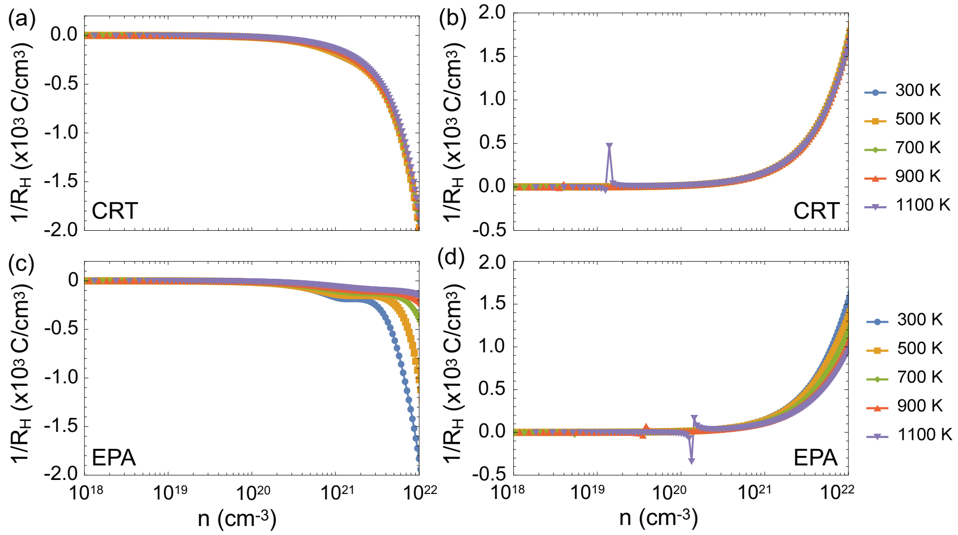


Figure 5. Inverse Hall coefficient $1/R_H$ of TaFeSb as a function of carrier concentration $n$, with colors labeling different temperatures. Panels (a) and (b) show $1/R_H$ for n-type and p-type TaFeSb calculated using the CRT approximation, panels (c) and (d) show $1/R_H$ of n-type and p-type TaFeSb calculated with the EPA approximation.

## B. ZrNiSn

Here we report on the estimates of the transport properties of ZrNiSn.

### 1. *CRT approximation*

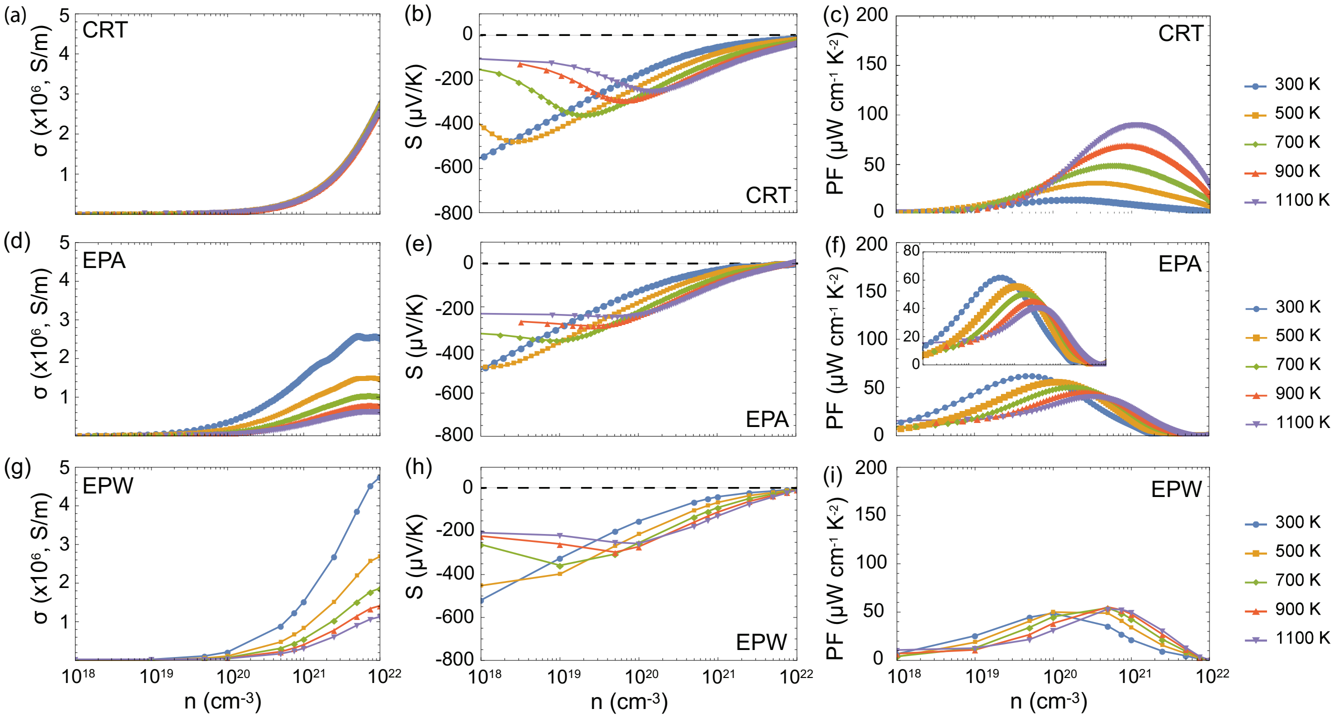


Figure 6. Electronic transport properties of n-type ZrNiSn as functions of carrier concentration $n$, i.e. electrical conductivity $\sigma$, Seebeck coefficient $S$ and power factor PF. The top row shows the predictions of the CRT approximation; middle row are estimates based on the EPA approximation, and the Wannier-interpolation estimates are in the bottom row. Various temperatures are highlighted in different colors.

First, we calculate the electrical conductivity $\sigma$, the Seebeck coefficient $S$ and the power factor PF of n-type ZrNiSn in the temperature range 300 - 1100 K and carrier concentrations range $10^{18}$ - $10^{22}$ cm$^{-3}$ using the CRT approximation, as shown in Fig. 6 in panels (a), (b) and (c), respectively. Generally, $\sigma$ gradually increases with electron doping concentrations and has a weak dependence on $T$. In turn, $|S|$ gradually decreases with $n$ and has a more pronounced temperature dependence. Unlike n-type TaFeSb discussed in the main text, we do not observe any increase in the absolute value of $S$ at large $n$. PF reaches its peak value of $\approx 90$ $\mu$W cm$^{-1}$ K$^{-2}$ at $n \approx 1.1 \times 10^{21}$ cm$^{-3}$ and $T = 1100$ K.

For p-type ZrNiSn we obtain similar qualitative behavior to that of n-type ZrNiSn for all aforementioned transport coefficients (except that $S$ has positive values for p-type systems), see Figs. 7 (a)-(c).

### 2. *EPA approximation*

First we comment on the EPA estimates of transport coefficients for n-type ZrNiSn shown in Figs. 6 (d)-(f). In contrast to the CRT approximation, here $\sigma$ exhibits a more pronounced temperature dependence, thanks to the more accurate description of electron-phonon scattering. Unlike n-type TaFeSb, the electrical conductivity of n-type ZrNiSn doesn't have a peak with respect to the doping concentration. $S$ shows a similar behavior to that predicted by the CRT approximation (Fig. 6 (b)) within the range of carrier concentrations considered here and doesn't show the anomalous change in sign. The PF reaches a peak value of 62 $\mu$W cm$^{-1}$ K$^{-2}$ at $n \approx 5 \times 10^{19}$ cm$^{-3}$ and at $T = 300$ K, and we note that both temperature dependence and doping dependence of such peak is significantly different from the CRT prediction.

The transport properties of p-type ZrNiSn calculated using the EPA approximation are shown in Fig. 7 (d)-(f). Here, $\sigma$ shows the anomalous peak similar to that found for n-type TaFeSb (Fig. 1 (d) of the main text). In the same manner, also $S$ shows the anomalous change in sign taking place at large doping concentrations. Finally, we also find the anomalous presence of two peaks in the PF discussed in the main text. Here we highlight how the CRT approximation (Fig. 7 (c)) doesn't capture the PF features described by the EPA method, with notable discrepancies in both carrier doping concentration and temperature dependences. In fact, CRT and EPA predict opposite temperature dependencies of the PF, with the EPA predicting higher PF at lower temperatures, and the CRT predicting an increasing PF with temperature.

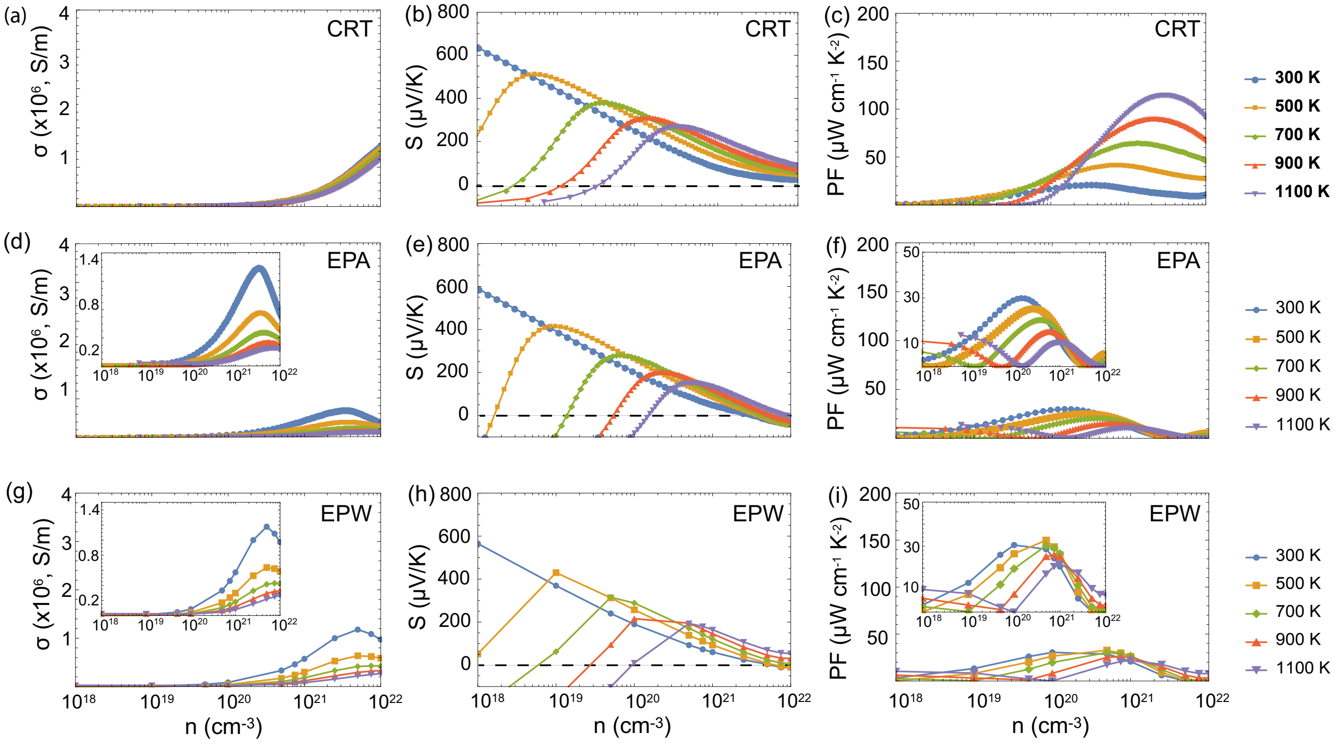


Figure 7. Electronic transport properties (the electrical conductivity $\sigma$, the Seebeck coefficient $S$, and the power factor PF) of p-type ZrNiSn as functions of carrier concentration $n$ at various temperatures (color-labelled). Panels (a-c) show predictions obtained using the CRT approximation, panels (d-f) show results for the EPA approximation, and panels (g-i) - for the Wannier-interpolation method.

### 3. *EPW method*

Finally, we employ the Wannier-interpolation method to estimate the electronic transport coefficients of ZrNiSn. The obtained $\sigma$, $S$ and PF of n-type and p-type ZrNiSn are presented in Figs. 6 (g-i) and 7 (g-i), respectively. We stress that the Wannier-interpolation method validates the EPA approximation, as it reproduces the qualitative behavior of the quantities considered here as functions of temperature and carrier concentrations. In particular, the anomalous behavior of $\sigma$ and $S$ of p-type ZrNiSn at high carrier concentrations is confirmed by the EPW method, and it is not found for n-type ZrNiSn. However, it's worth noting that EPW predicts approximately twice larger electrical conductivity for n-type ZrNiSn compared to the EPA prediction, likely caused by the more detailed wavevector dependence of the electron-phonon coupling. We observe instead a better quantitative agreement for p-type ZrNiSn.

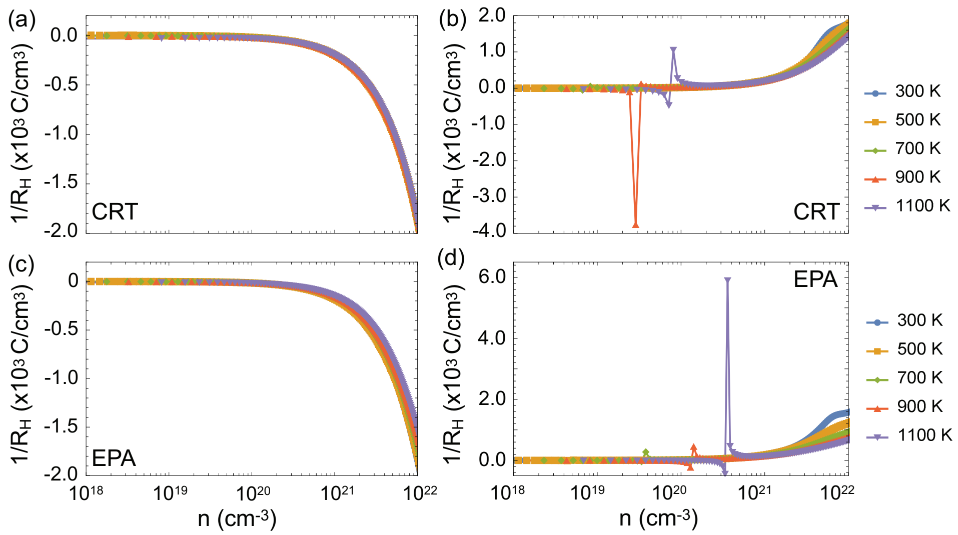


Figure 8. Inverse Hall coefficient $1/R_H$ of ZrNiSn as a function of carrier concentration $n$ for n-type and p-type ZrNiSn (left and right panels respectively), as predicted by the CRT and EPA approximations (top and bottom panels respectively). Different colors of curves correspond to different temperatures in the range 300 - 1100 K. We point out that even in conditions when the Seebeck coefficient changes sign as a function of the doping concentration, the Hall coefficient maintains the same sign.

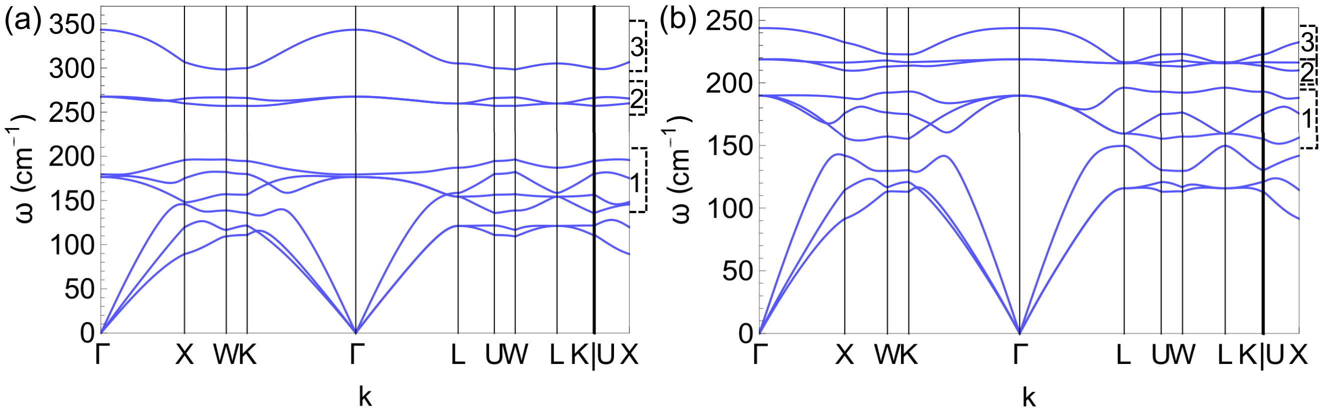


Figure 9. Calculated phonon dispersion of (a) TaFeSb and (b) ZrNiSn. For each material, we identify three groups of optical phonon branches (shown to the figure's right side). The phonon frequencies of these groups have been averaged and used for estimating electron-phonon scattering in the two-parabolic-bands model. Similarly, the remaining acoustic modes are averaged as an additional group.

## IV. ORIGIN OF THE ANOMALOUS BEHAVIOR OF TRANSPORT COEFFICIENTS IN HALF-HEUSLER SYSTEMS

### A. TaFeSb

In this section we show additional results of the two parabolic band model discussed in the main text.

In Fig. 9 (a) we show the phonon dispersion relations. We identified four groups of phonon bands (one acoustic and three optical groups). These groups of phonon energies have been averaged (finding 75, 175, 270 and 325 $\mathrm{cm}^{-1}$) and used as the phonon energies entering the EPA estimate of lifetimes for the two-parabolic-band model.

In Fig. 10 we plot results for TaFeSb obtained within the CRT approximation (top row) and the EPA model (bottom row). However, in the EPA estimate of lifetimes we only included intraband scattering. As evident in the picture, the absence of interband scattering causes a suppression of the anomalous behavior of transport coefficients discussed in the main text.

In Fig. 11 we plot the transport properties of TaFeSb obtained using the two-parabolic-band model; however,

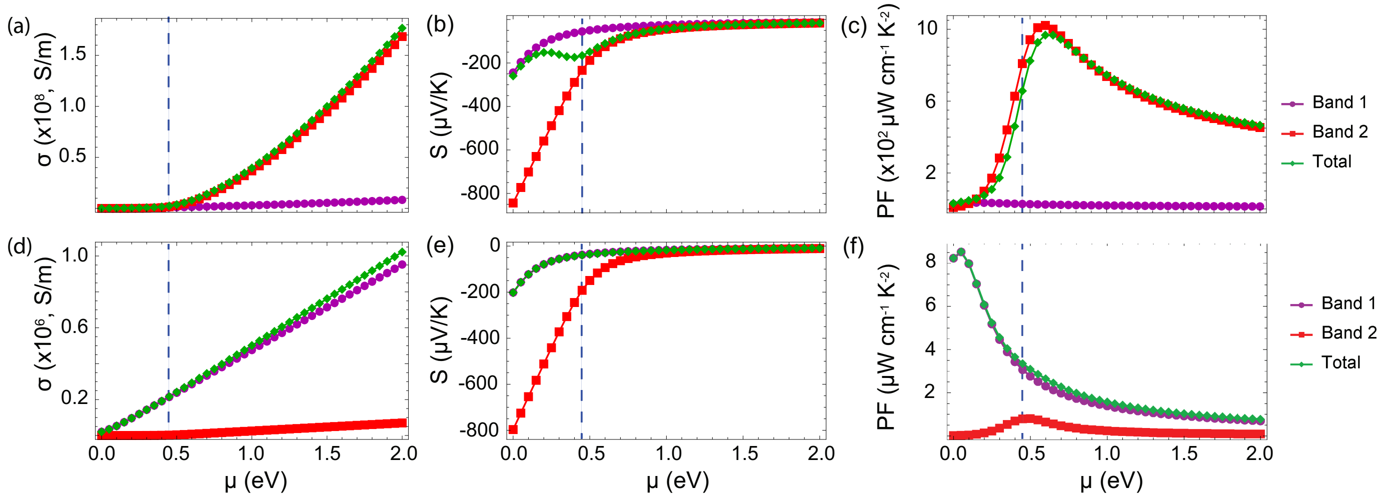


Figure 10. Electronic transport properties of n-type TaFeSb calculated using the two-parabolic-bands model as functions of chemical potential $\mu$ at $T = 700$ K. The dashed line marks the energy of the bottom of the higher energy band ($\mu = E_{0,2}$). The top row shows CRT predictions ($\tau = 10$ fs) for the transport coefficients; and the bottom row shows results using an energy dependent lifetime restricted to only intravalley scattering. Panels (a) and (d) show the electrical conductivity $\sigma$, panels (b) and (e) show the Seebeck coefficient $S$, panels (c) and (f) show the power factor PF.

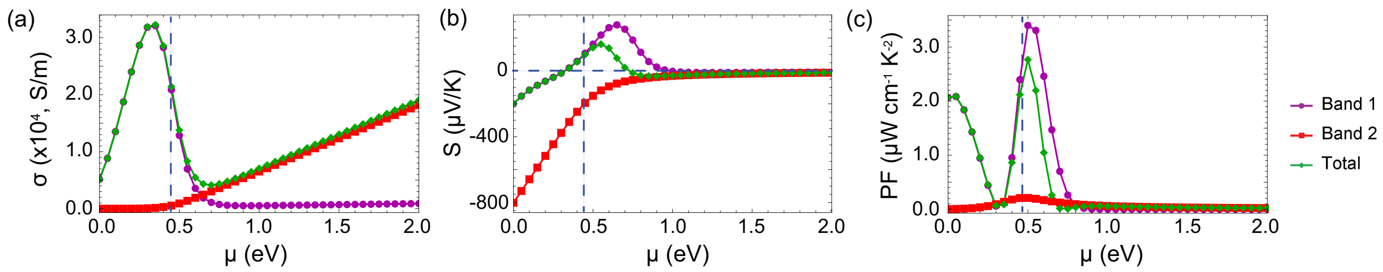


Figure 11. Electrical conductivity $\sigma$, Seebeck coefficient $S$ and power factor PF of n-type TaFeSb at 700K as functions of the chemical potential $\mu$, calculated using the two-parabolic-bands model and a simplified expression for the energy dependent electron lifetime: $\tau(E) = g_s\hbar/(2\pi\Omega\rho(E)g^2)$ (where $\Omega$ is the unit cell volume, $g_s = 2$ the spin degeneracy, $\hbar$ the reduced Planck constant, and $\rho(E)$ the electronic density of states. The averaged squared value of the electron-phonon matrix elements $g^2$ is set to 1 eV$^2$. The vertical dashed line indicates the energy of the bottom of the higher energy band ($\mu = E_{0,2}$).

lifetimes $\tau$ are calculated using an even simpler estimate, namely that $\tau(E) \propto 1/\rho(E)$, where $\rho$ is the density of states.

Lastly, Fig. 12 shows an analysis of the electrical conductivity predicted by the two-band-parabolic model for n-type TaFeSb, explaining how the suppression of lifetime is connected to the origin of the peak in electrical conductivity.

### B. ZrNiSn

In this section we describe the set of parameters which have been used to calculate the electronic transport properties of n-type ZrNiSn using two-parabolic-bands model (the results are shown in Fig. 5 of the main text).

In ZrNiSn the conduction band edge is represented by a single valley with the minimum at $X$ point and the degeneracy $N_v = 3$ (see Fig. 2 (b) of the main text). At higher energies, there are two lighter valleys at $K$ and $U$ points ($N_v = 12$ in both cases). Therefore, in the two-parabolic-bands model calculations we set $N_1 = 3$ for a lower energy band and $N_2 = 24$ for a higher energy (two higher energy valleys at $K$ and $U$ points in the DFT band structure are approximated as a single band with the degeneracy $N_2 = N_{v,1} + N_{v,2} = 24$). The averaged value of squared electron-phonon matrix elements is set to $g^2 = 0.0064$ eV$^2$ based on the results of full EPA calculations; for all acoustic phonon modes we use $\bar{\omega} = 75$ cm$^{-1}$ and for the groups of optical phonons denoted as 1, 2 and 3 in 9 (b) we set $\bar{\omega} = 175$, 220 and 235 cm$^{-1}$, respectively.

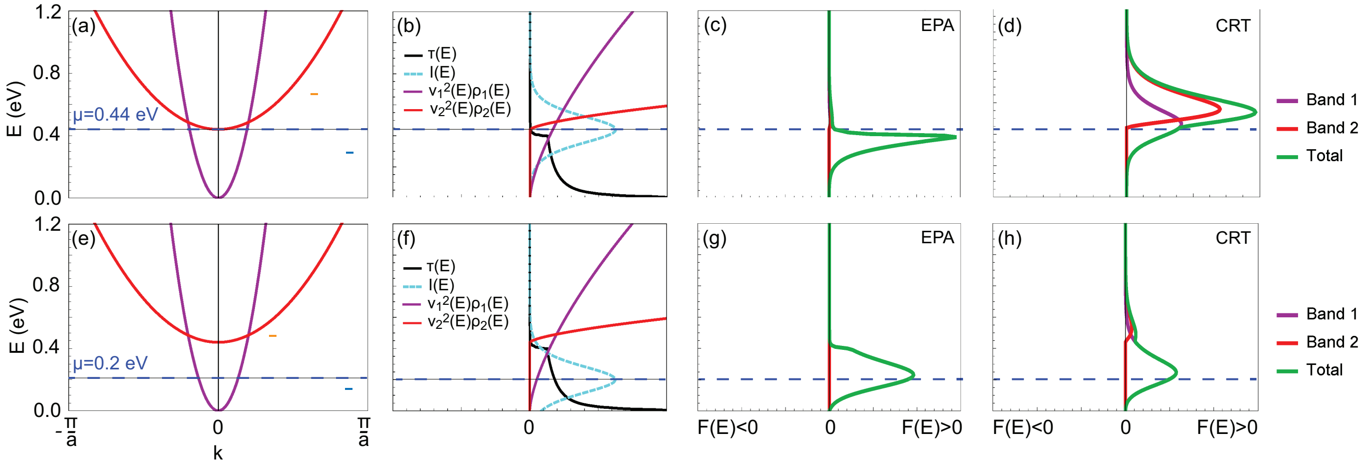


Figure 12. Analysis of the anomalous reduction of the electrical conductivity $\sigma$ for n-type TaFeSb at high doping concentrations using the two-parabolic-bands model. Top row: analysis of $\sigma$ when the chemical potential is at the minimum of the higher-energy band. Bottom row analyzes the case where the chemical potential lies below the second band minimum. Panels (a) and (e) show the model band structures, with the chemical potential $\mu$ indicated by the dashed line. Panels (b) and (f) show the different contributions to $\sigma$, such as density-of-state projected velocity $v^2\rho$, electron lifetime $\tau(E)$ and function $I^{(0)}(E,\mu,T) = f(E,\mu,T)[1-f(E,\mu,T)]$ which acts as a filter that activates only electrons within a few $k_BT$ of the chemical potential ($f(E,\mu,T)$ is the Fermi-Dirac distribution function). Note in particular that the sharp increase in $v^2\rho$ at $E \approx 0.5$ eV is counterbalanced by a sharper decrease in the relaxation time $\tau$, which effectively suppresses $\sigma$. Next, we show the energy and band resolved contributions to the integrands $F_1(E)$, $F_2(E)$ and $F(E)$ which define $\sigma$ (see the integrand in Eq. (2) of the main text), calculated within the EPA (panels (c) and (g)) or CRT approximations (panels (d) and (h)). Thanks to the energy dependence of $\tau$, the EPA can capture the suppression of $\sigma$ taking place at high energies. The CRT instead neglects this suppression and only takes into account for a larger density of states. The scattering of electrons by phonons is therefore of critical importance for describing even the qualitative features of transport.

### C. Band convergence

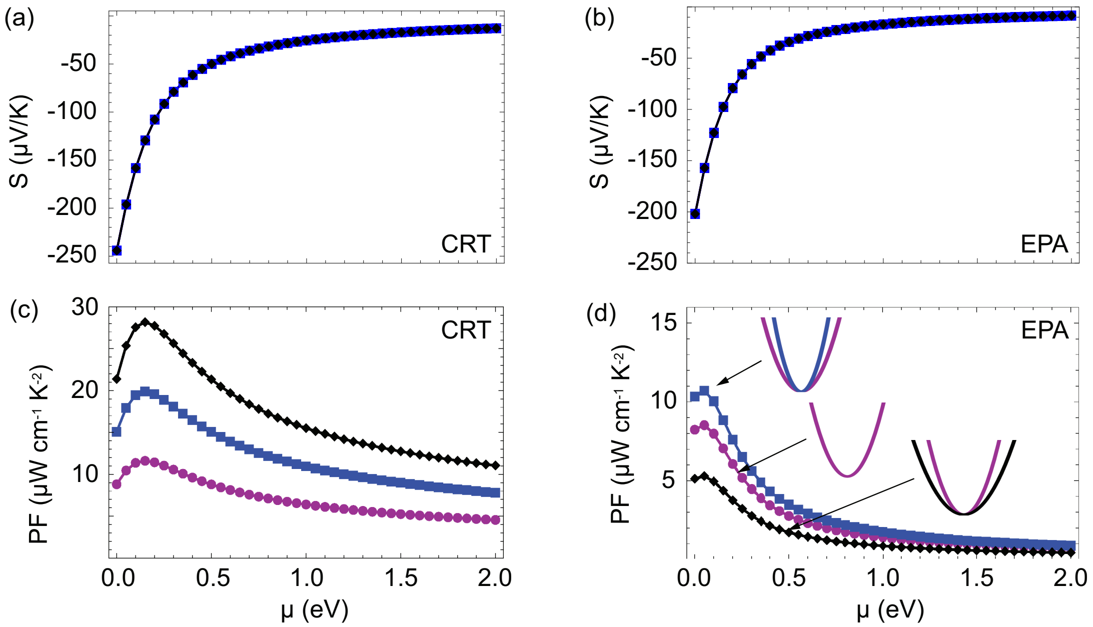


Figure 13. Change to Seebeck coefficient $S$ and power factor PF upon adding a light or heavy band on top of an existing band with the same energy minimum, estimated at a temperature of 700 K as a function of the chemical potential $\mu$. In purple color we show $S$ and PF for a system with a single band. In black and blue, the resulting $S$ and PF after adding a heavier or lighter band respectively. In the panels (a) and (b), we show the predictions for $S$ from CRT and EPA approximations, respectively. Both approximations predict no effect on $S$ by converging a single band with an extra band (light or heavy). In panel (c) we show the CRT prediction for PF, according to which band convergence improves PF and the effect is larger if a single band is converged with a heavier band. This is due to increase in the electrical conductivity $\sigma$ achieved by band convergence as it is shown in Fig. 6 (a) of the main text. In panel (d) we show the EPA prediction for PF, according to which PF is improved by adding a lighter band, while it is reduced by adding heavier band following the behavior of the electrical conductivity upon band convergence as shown in Fig. 6 (b) of the main text.

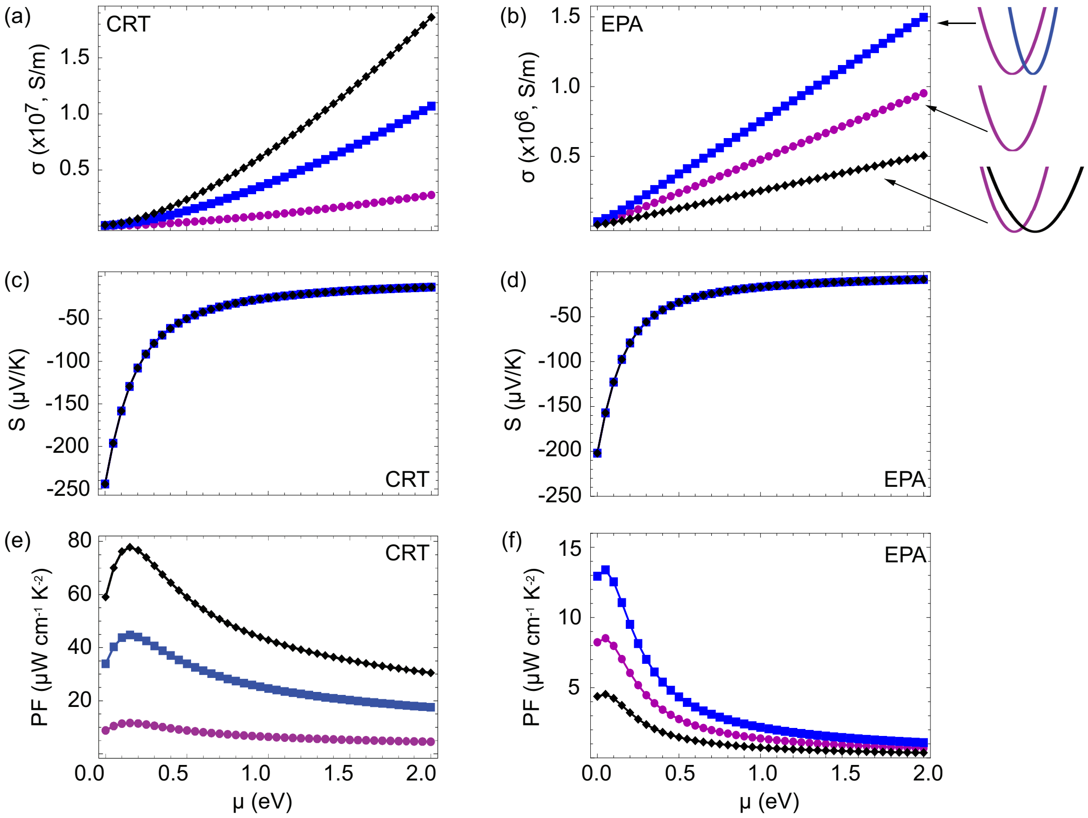


Figure 14. Values of electrical conductivity $\sigma$, Seebeck coefficient $S$ and power factor PF for three scenarios. Purple color: the system has a single "reference" parabolic band 1. Black color: we add to the system a heavier band "2". Blue color: we add to the system a lighter band "2". These cases are also shown to the right of panel (b). Making the hypothesis that the minima of the bands occur at different points of the Brillouin zone, we can set different degeneracies, specifically $N_1 = 1$ and $N_2 = 4$ for the two bands. The transport coefficients are estimated at a temperature of 700 K and plotted as functions of the chemical potential $\mu$. The left column shows predictions obtained using the CRT approximation, and are contrasted to the EPA predictions to the right. The Seebeck coefficient does not change in these scenarios and is reproduced by both EPA and CRT methods. CRT and EPA predictions disagree for electrical conductivity. In fact, CRT predicts that adding a heavy band leads to an increase of conductivity compared to the other cases, and it is a result of over weighting the contribution to $\sigma$ from the density of states. The EPA result shown in panel (b) instead demonstrates that adding a light band leads to an increase of $\sigma$, while adding a heavy band results in a decrease, as one would expect due to the presence of slower electrons. In the bottom row we see that the qualitatively different predictions on $\sigma$ propagate to the PF, with the CRT predicting that adding a heavy band leads to better power factors, whereas EPA predicts the opposite behavior and the best performance by adding a lighter band.

## V. MATERIALS DESIGN RULES

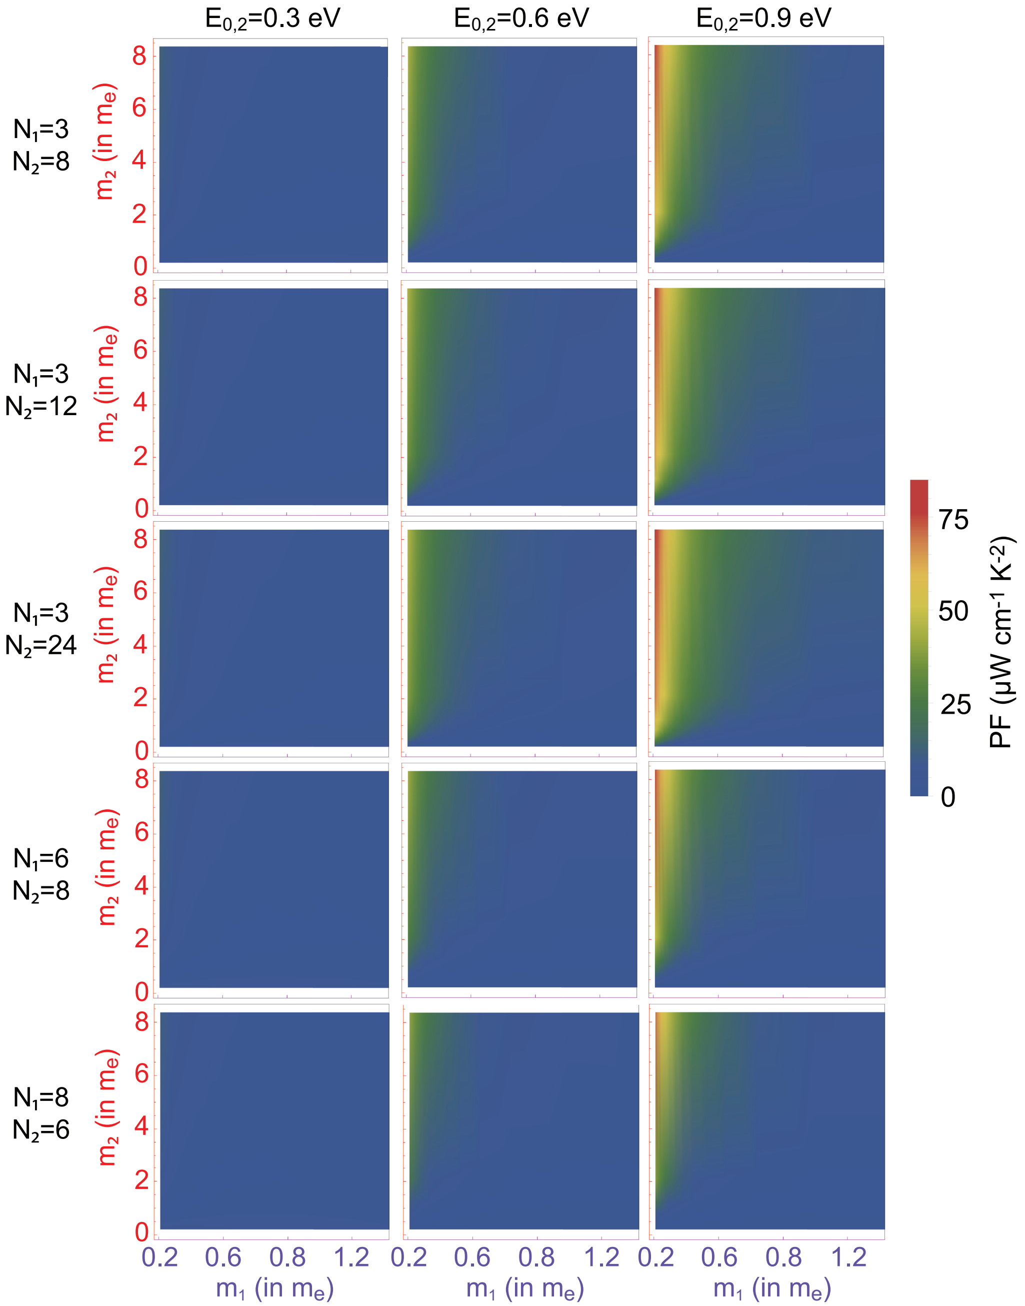


Figure 15. Magnitude of the anomalous peak in the power factor (PF) as a function of the band effective masses $m_1$ and $m_2$, as predicted by the two-parabolic-bands model. PF values correspond to the chemical potential $\mu$ placed exactly at the extremum of the higher energy band ($\mu = E_{0,2}$). For each row in figure we change the degeneracies of the two bands ($N_1$ and $N_2$, respectively), showing that it is preferable to have $N_2 > N_1$ . Each column corresponds to different band offset values $E_{0,2}$ (i.e. the position of the extremum of the higher-energy band with respect to the extremum of the lower-energy band), showing that it is preferable to have a large energy difference between the two bands. It's worth noting however that larger offset require larger doping concentrations to reach such anomalous PF peak.

* natalya.fedorova@list.lu
† bkoz@seas.harvard.edu

[1] W. Kohn and L. J. Sham, Phys. Rev. **140**, A1133 (1965).
[2] P. Hohenberg and W. Kohn, Phys. Rev. **136**, B864 (1964).
[3] S. Baroni, S. de Gironcoli, A. Dal Corso, and P. Giannozzi, Rev. Mod. Phys. **73**, 515 (2001).
[4] P. Giannozzi, S. Baroni, N. Bonini, M. Calandra, R. Car, C. Cavazzoni, D. Ceresoli, G. Chiarotti, M. Cococcioni, I. Dabo, et al., Journal of Physics: Condensed Matter **21**, 395502 (2009).
[5] P. Giannozzi, O. Andreussi, T. Brumme, O. Bunau, M. B. Nardelli, M. Calandra, R. Car, C. Cavazzoni, D. Ceresoli, M. Cococcioni, et al., Journal of Physics: Condensed Matter **29**, 465901 (2017).
[6] J. P. Perdew, K. Burke, and M. Ernzerhof, Phys. Rev. Lett. **77**, 3865 (1996).
[7] D. R. Hamann, Phys. Rev. B **88**, 085117 (2013).
[8] H. Zhu, J. Mao, Y. Li, J. Sun, Y. Wang, Q. Zhu, G. Li, Q. Song, J. Zhou, Y. Fu, et al., Nature Communications **10**, 270 (2019), ISSN 2041-1723.
[9] J. Schmitt, Z. M. Gibbs, G. J. Snyder, and C. Felser, Mater. Horiz. **2**, 68 (2015).
[10] G. Madsen and D. J. Singh, Computer Physics Communications **175**, 67 (2006).
[11] G. Samsonidze and B. Kozinsky, Advanced Energy Materials **8**, 1800246 (2018).
[12] S. Bang, J. Kim, D. Wee, G. Samsonidze, and B. Kozinsky, Materials Today Physics **6**, 22 (2018).
[13] F. Giustino, M. L. Cohen, and S. G. Louie, Phys. Rev. B **76**, 165108 (2007).
[14] J. Noffsinger, F. Giustino, B. D. Malone, C.-H. Park, S. G. Louie, and M. L. Cohen, Computer Physics Communications **181**, 2140 (2010).
[15] S. Ponce, E. Margine, C. Verdi, and F. Giustino, Computer Physics Communications **209**, 116 (2016).
